# Supplementary material for: Operational route planning under uncertainty for Demand Adaptive Systems
Source: arXiv:2503.07812 source file (2025-03-10)
Supplement: Supplementary file 1 [file appendix.tex]

\section{Appendix}
